# Supplementary material for: Microtubule catastrophe from protofilament dynamics
Source: arXiv:1308.5778 source file (2013-09-19)
Supplement: Supplementary file 1 [file supplement.pdf]

# Supplementary material for the paper 'Microtubule catastrophe from protofilament dynamics'

V. Jemseena and Manoj Gopalakrishnan

Details of calculation of protofilament catastrophe in the steady state studied under various condition are given. General expressions for the relevant probabilities are derived in the appendix.

## 1 Non-zero rescue and $k_h > 0$

### 1.1 $k_g > k_h$

In order to identify steady state expressions for the required probabilities and there by the protofilament catastrophe frequency, we utilize the following small $s$-expansions for $z_1$ and $z_2$ in this regime (obtained from A.4):

$$z_1 = \frac{k_h}{k_g}\left[1 - \frac{s}{(k_g - k_h)}\right] \quad ; \qquad z_2 = 1 + \frac{s}{(k_g - k_h)}. \tag{S1}$$

We find that the only non-zero steady state contribution comes from $\tilde{P}_1^{(1)}(s)$ which in turn gives the steady state expression for $\tilde{P}_1^{(1)}(s)$ as

$$\tilde{P}_1^{(1)}(s) \simeq \frac{2k_g k_h - k_h^2}{s k_h (k_g - k_h)^2}. \tag{S2}$$

From Eq.9 in the main text, we thus find that $\nu_c'$ does not have a zero'th order term, and the first order term is given by

$$\nu_c' = r k_h P_1^{(1)}. \tag{S3}$$

which gives Eq.10 in the main text.

### 1.2 $k_g < k_h$

In this regime $z_1$ and $z_2$ take the following forms as $s \to 0$:

$$z_1 = 1 + \frac{s}{(k_g - k_h)} \quad ; \qquad z_2 = \frac{k_h}{k_g}\left[1 - \frac{s}{(k_g - k_h)}\right], \tag{S4}$$

which can be used to identify the steady state limits of the probabilities. By substitution, we get the following steady state expressions

$$\tilde{P}_0^{(0)}(s) = \frac{(k_h - k_g)}{s(k_h + \nu_r' - k_g)} \quad ; \qquad \tilde{P}_1^{(0)}(s) = \frac{\nu_r'(k_h - k_g)}{s k_h (k_h + \nu_r' - k_g)}, \tag{S5}$$

$$\tilde{P}_0^{(1)}(s) = \frac{k_g(k_h-k_g)}{s(k_h+\nu_r'-k_g)}\Bigg\{\frac{k_g}{(k_h-k_g)^3}+\frac{1}{(k_h-k_g)^2}$$
$$+\frac{(\nu_r'-k_g)}{k_g(k_h-k_g)(k_h+\nu_r'-k_g)}+\frac{(\nu_r'-k_g)}{(k_g-k_h)^2(k_h+\nu_r'-k_g)}\Bigg\}, \quad (S6)$$

$$\tilde{P}_1^{(1)}(s) = \frac{\nu_r'}{sk_h}\Bigg[\frac{k_g(k_h-k_g)}{(k_h+\nu_r'-k_g)}\Bigg\{\frac{k_g}{(k_h-k_g)^3}+\frac{1}{(k_h-k_g)^2}$$
$$+\frac{(\nu_r'-k_g)}{k_g(k_h-k_g)(k_h+\nu_r'-k_g)}+\frac{(\nu_r'-k_g)}{(k_g-k_h)^2(k_h+\nu_r'-k_g)}\Bigg\}$$
$$-\frac{1}{(k_h+\nu_r'-k_g)}\Bigg]. \quad (S7)$$

After substitution of the above results in Eq.9 in the main text, we reach the result in Eq.12 in the main text.

# 2 One dimensional continuum FHL model solved using perturbative method

In section IV B of the main text, we had mentioned the similarity between Eq.14 and the corresponding result in the continuum model of Flyvbjerg, Holy and Leibler [7]. In this section, we present a derivation of this result using our perturbative approach. In the continuum model, where the microtubule as a whole is taken as one dimensional linear polymer, the dynamics of the cap, specified by the probability distribution $P(x,t)$ for cap length $x$ at time $t$, is given by the partial differential equation,

$$\frac{\partial P(x,t)}{\partial t} = D_0\frac{\partial^2 P(x,t)}{\partial x^2} - v\frac{\partial P(x,t)}{\partial x} - r'\left[xP(x,t) - \int_x^\infty P(y,t)dy\right], \quad (S8)$$

where

$$2D_0 = (k_g+k_h)\delta x^2 \quad ; \quad v = v_g - v_h,$$

and $r'$ is the rate at which spontaneous hydrolysis takes place per unit length of the GTP cap, and $\delta x$ is the length of an effective monomer unit. Although Eq.$S8$ can be solved exactly [7], we attempt a perturbation theory solution here, by expanding $P(x,t)$ in powers of $r'$:

$$P(x,t) = P^{(0)}(x,t) + r'P^{(1)}(x,t) + (r')^2P^{(2)}(x,t) + \dots \quad (S9)$$

After substitution of Eq.$S9$, for terms up to $O(r')$, Eq.$S8$ splits into two partial differential equations

$$\frac{\partial P^{(0)}(x,t)}{\partial t} = D_0\frac{\partial^2 P^{(0)}(x,t)}{\partial x^2} - v\frac{\partial P^{(0)}(x,t)}{\partial x},$$
$$\frac{\partial P^{(1)}(x,t)}{\partial t} = D_0\frac{\partial^2 P^{(1)}(x,t)}{\partial x^2} - v\frac{\partial P^{(1)}(x,t)}{\partial x} - xP^{(0)}(x,t) + \int_x^\infty P^{(0)}(y,t)dy. \quad (S10)$$

In the continuum model, the catastrophe frequency is defined as

$$\nu_c^{FHL}(t) = \frac{D_0 \partial_x P(x,t)|_{x=0}}{\int_0^\infty P(x,t)dx}. \tag{S11}$$

We solved Eq.$S10$ using Laplace transforms as we did in the discrete case, subject to the initial conditions $P^{(0)}(x, t = 0) = \delta(x - \lambda)$ and $P^{(1)}(x, t = 0) = 0$, where $\lambda$ is an arbitrary initial length of the cap. The solutions, to $O(r)$ are given as

$$\tilde{P}^{(0)}(k,s) = \frac{D_0 \alpha^0(s) - \exp(-k\lambda)}{D_0(k - k_0'))(k + k_0)} \tag{S12}$$

and

$$\tilde{P}^{(1)}(k,s) = \frac{D_0 \alpha^1(s) - \tilde{F}(k,s)}{D_0(k - k_0')(k - k_0)}, \tag{S13}$$

where

$$\alpha^0(s) = \partial_x \tilde{P}^{(0)}(x,s)|_{(x=0)} \quad ; \quad \alpha^1(s) = \partial_x \tilde{P}^{(1)}(x,s)|_{(x=0)}, \tag{S14}$$

and the constants $k_0$ and $k_0'$ are given by

$$\begin{aligned} k_0 &= -\frac{(v_g - v_h)}{2D_0} + \sqrt{\frac{s}{D_0} + \frac{(v_g - v_h)^2}{4D_0^2}}, \\ k_0' &= \frac{(v_g - v_h)}{2D_0} + \sqrt{\frac{s}{D_0} + \frac{(v_g - v_h)^2}{4D_0^2}}. \end{aligned} \tag{S15}$$

The function $\tilde{F}(k,s)$ appearing in Eq.$S13$ is the double transform of $F(x,t)$, i.e., $F(k,s) = \int_0^\infty \int_0^\infty \exp(-st) \exp(-kx) F(x,t) dx\ dt$, where $F(x,t)$ is defined as

$$F(x,t) = -xP^{(0)}(x,t) + \int_x^\infty P^{(0)}(y,t)dy, \tag{S16}$$

with the above definition, the transform turns out to be

$$\tilde{F}(k,s) = \frac{\partial \tilde{P}^{(0)}(k,s)}{\partial k} + \frac{1}{k}\left[\tilde{P}^{(0)}(k=0,s) - \tilde{P}^{(0)}(k,s)\right]. \tag{S17}$$

After substituting Eq.$S15$ and Eq.$S17$ into Eq.$S13$, we do the inverse transformation $k \to x$, which yields terms that diverge or decay with $x$ exponentially, as $x \to \infty$. The first set of terms are now put to zero, on account of the requirement of convergence of the integral $\int P(x,t)dx$. This procedure therefore fixes the constants $\alpha^0(s)$ and $\alpha^1(s)$ respectively as

$$\alpha^0(s) = \frac{\exp(-k_0'\lambda)}{D_0} \quad ; \quad \alpha^1(s) = \frac{\tilde{F}(k_0', s)}{D_0}. \tag{S18}$$

Using the above results in the definition in Eq.$S11$ yields the steady state result in Eq.11 in the main text.

# 3 Zero rescue, $\nu_r' = 0$

## 3.1 $k_g > k_h$, $k_h > 0$

In this limit, the explicit expression for $\tilde{P}_0^{(0)}(s)$ and $\tilde{P}_0^{(1)}(s)$ in the Laplace space are obtained by putting $\nu_r' = 0$ in Eq.$A$.12-Eq.$A$.13 in the main text:

$$\tilde{P}_0^{(0)}(s) = \frac{z_1^{N+1}}{(k_h - k_g z_1)(1 - z_1)}. \tag{$S19$}$$

$$\begin{aligned}
\tilde{P}_0^{(1)}(s) = \frac{1}{(1-z_1)(z_2-1)} \Bigg[ & \frac{(1-z_1^N)}{k_g^2(z_2-z_1)(1-z_1)^2} - \frac{N z_1^N}{k_g^2(z_2-z_1)(1-z_1)} \\
& + \frac{z_1^{N+1}(k_h - k_g z_2)}{k_g^2(k_h - k_g z_1)(1-z_1)(z_2-z_1)^2} + \frac{1}{k_g^2(z_2-z_1)(z_2-1)(1-z_1)} \\
& - \frac{z_1^{N+1}}{k_g^2(z_2-z_1)^2(1-z_1)} - \frac{z_1^{N+2}}{k_g^2(z_1-z_2)^2(1-z_1)} - \frac{(N+1)z_1^{N+1}}{k_g^2(z_1-z_2)^2} \\
& + \frac{N(N+1)z_1^N}{2k_g^2(z_1-z_2)} - \frac{z_1^{N+2}}{k_g(z_1-z_2)^2(k_h-k_g z_1)} \\
& - \frac{z_1^{N+2}}{k_g(z_1-z_2)(1-z_1)(k_h-k_g z_1)} \Bigg].
\end{aligned} \tag{$S20$}$$

where $z_1$ and $z_2$, in the $s \to 0$ limit, are given by Eq.$S$1. After substitution of $z_1$ and $z_2$, it turns out that only $\tilde{P}_0^{(0)}(s)$ and $\tilde{P}_1^{(1)}$ ($\tilde{P}_1^{(1)}$ is evaluated using Eq.7 in the main text from Eq.$A$.12 by putting $\nu_r'$=0) have non-zero steady state values, given as follows

$$\tilde{P}_0^{(0)}(s) = \frac{1}{s}\left(\frac{k_h}{k_g}\right)^N \quad ; \quad \tilde{P}_1^{(1)}(s) = \frac{1}{s(k_g - k_h)(1 - (\frac{k_h}{k_g})^N)}. \tag{$S21$}$$

The substitution of these values in the relevant equation

$$\nu_c' = \frac{r k_h P_1^{(1)}}{1 - P_0^{(0)}}, \tag{$S22$}$$

derived from Eq.9 gives Eq.14 in the main text. A few points may be noted here. From Eq.1 in the main text, it is easy to see that when $\nu_r' = 0$, the only formal steady state solution possible is $P_m = 0$ for all $m \geq 1$, and hence, by normalization, $P_0 = 1$. Our expression for $P_0^{(0)}$ above does not contradict this assertion, as it refers to $r = 0$. Therefore, the higher order terms in $P_0(t)$ and $P_1(t)$ (and also all $P_m(t)$ with $m > 1$)should necessarily have terms that individually diverge with $t$ as $t \to \infty$. An advantage of the perturbative approach in $r$, as we have used in this paper, is that, in spite of this, we are able to derive the steady state result for $\nu_c'$, which is otherwise difficult (as it would lead to a 0/0 situation in Eq.2 in the main text).
